# Supplementary material for: MEGAN: Memory Enhanced Graph Attention Network for Space-Time Video Super-Resolution
Source: arXiv:2110.15327 source file (2021-11-30)
Supplement: Supplementary file 1 [file appendix.tex]

In this supplementary material, we provide further comparisons to investigate the effects of different components in MEGAN.

%  reports details on our pris-tine data acquisition
% first show the influence of the temperature parameter for inference in Sec. 1. Secondly, we present additional details about the minimally generalized L1 loss in Sec. 2. Third, we provide a further qualitative and quantitative comparison of AdFlow with other state-of-the-art methods in Sec. 3. Finally, we show more visual results for the DIV2K dataset in Sec. 
\section{More Ablation Study}
\subsection{More analysis on different components}
We conduct experiments of MEGAN w/o GCN, MEGAN w/o non-local, MEGAN w/o global-local feature aggregation (GL-Agg). In the table below, results show that the proposed method \textbf{achieved significant improvements} over i).~w/o GCN, ii).~w/o NLRB, or iii).~w/o GL-Agg. This proved the effectiveness of each component.

\subsection{Further analysis on attention-based blocks and LMGA}
% \noindent\textbf{Non-local Mixed Attention}. 
In Table \ref{tab:results_ablation_component}, when comparing cases 1-3, we use different types of attention blocks (Channel-based Attention Block \cite{zhang2018image}, Non-local Block \cite{wang2018non}, and Non-local Resblock \cite{yi2019progressive}) instead of the proposed LMGA module. We can observe that the non-local module brings performance improvements. This suggests that, by exploiting low-level and high-level features, MEGAN is capable of utilizing non-local information to learn better representational ability. In case 4, we also learn that the proposed LMGA block contributes to superior performance gains, regardless of whether we use attention-based blocks (cases 1-3). This demonstrates that we can significantly improve the reconstruction performance in space-time domain by dynamically incorporating information from spatial features and temporal contexts.

We fix the proposed LMGA in MEGAN in cases 5-7. We observe that performance improvements benefit from utilizing Non-local Resblock, suggesting adopting residual non-local learning is able to capture long-range spatio-temporal correlations, which results in a marginal gain in network performance. Besides, residual learning \cite{he2016deep} is employed to promote the training process more stable.

\begin{table*}[htpb]
\scriptsize
%\footnotesize
%\small
%\normalsize
\centering
\begin{center}
%\caption{Ablation investigation of contiguous memory (CM), local residual learning (LRL), and global feature fusion (GFF). We observe the best performance (PSNR) on Set5 with scaling factor $\times2$ in 200 epochs.} 
\vspace{-5mm}

\caption{Ablation study of different components on Vid4 \cite{liu2011bayesian}.}
\label{tab:results_ablation_component}
%\vspace{-3mm}
%\begin{tabular*}{82.4mm}{@{\extracolsep{-0.75mm}}|c|c|c|c|c|c|c|c|c|}
\begin{tabular}{|c|c|c|c|c|c|c|c|}
\hline
Case Index & 1 & 2 & 3 & 4 & 5 & 6 & 7
%Combination Index & \multicolumn{8}{c|}{Different combinations} 
\\ 
\hline  
\hline
%\hline
Channel-based Attention Block~\cite{zhang2018image} & \Checkmark & \XSolid   & \XSolid & \XSolid & \Checkmark & \XSolid & \XSolid
\\
%\hline
Non-local Block~\cite{wang2018non} & \XSolid & \Checkmark   & \XSolid & \XSolid & \XSolid & \Checkmark & \XSolid
\\
Non-local Residual Module \cite{yi2019progressive} & \XSolid & \XSolid  & \Checkmark & \XSolid & \XSolid & \XSolid & \Checkmark
\\
LMGA & \XSolid & \XSolid & \XSolid & \Checkmark & \Checkmark & \Checkmark & \Checkmark
\\
\hline
% PFRDB Number & 5 & 5 & 10 & 20 & 30 & 10 & 10 & 10 & 10 & 10 & 10
% \\
% ResBlock Number & 20 & 20   & 20 & 20 & 20 & 0 & 5 & 10 & 15 & 20 & 30
% \\
% %\hline
% \hline
PSNR (dB) & 26.27 & 26.34 & 26.40 & 26.44 & 26.47 & 26.51 & 26.57
\\
% \hline
SSIM & 0.7985 & 0.7991 & 0.7999 & 0.0817 & 0.8018 & 0.8021 & 0.8044
\\
\hline
% Parameter Number & 30.96 & 31.17 & 31.20 & 31.32 & 30.78 & 30.99 & 31.27 & 31.50 & 30.99 & 31.27 & 31.50
% \\
% \hline
\end{tabular}
\end{center}
\vspace{-5mm}
\end{table*}

\begin{table*}[htpb]
\scriptsize
%\footnotesize
%\small
%\normalsize
\centering
\begin{center}
%\caption{Ablation investigation of contiguous memory (CM), local residual learning (LRL), and global feature fusion (GFF). We observe the best performance (PSNR) on Set5 with scaling factor $\times2$ in 200 epochs.} 
\vspace{-5mm}

\caption{Ablation study of block number on Vid4 \cite{liu2011bayesian}.}
\label{tab:results_ablation}
%\vspace{-3mm}
%\begin{tabular*}{82.4mm}{@{\extracolsep{-0.75mm}}|c|c|c|c|c|c|c|c|c|}
\begin{tabular}{|c|c|c|c|c|c|c|c|c|c|c|c|c|c|}
\hline
Case Index & 1 & 2 & 3 & 4 & 5 & 6 & 7 & 8 & 9 & 10
%Combination Index & \multicolumn{8}{c|}{Different combinations} 
\\ 
\hline  
% \hline
% LMGA & \XSolid & \Checkmark & \XSolid & \Checkmark & \Checkmark & \Checkmark & \Checkmark & \Checkmark & \Checkmark & \Checkmark & \Checkmark
% \\
% %\hline
% Channel-based Attention Block~\cite{zhang2018image} & \XSolid & \XSolid   & \Checkmark & \Checkmark & \Checkmark & \Checkmark & \Checkmark & \Checkmark & \Checkmark & \Checkmark & \Checkmark
% \\
\hline
PFRDB Number & 0 & 5 & 10 & 20 & 30 & 5 & 5 & 5 & 5 & 5
\\
ResBlock Number & 20 & 20 & 20 & 20 & 20 & 0 & 5 & 10 & 15 & 30
\\
%\hline
\hline
PSNR (dB) & 26.45 & 26.57 & 26.57 & 26.58 & 26.58 & 26.39 & 26.46 & 26.50 & 26.54 & 26.57
\\
% \hline
SSIM & 0.8024 & 0.8044 & 0.8045 & 0.8047 & 0.8045 & 0.8008 & 0.8012 & 0.8021 & 0.8028 & 0.8045
\\
\hline
Parameter Number & 10.01M & 10.71M & 11.41M & 12.80M & 14.20M & 9.23M & 9.60M & 9.97M & 10.34M & 11.46M
\\
\hline
\end{tabular}
\end{center}
\vspace{-5mm}
\end{table*}

\subsection{Further analysis on block number}
In this section, we conduct extensive experiments to investigate the effects of block number in MEGAN. When comparing cases 1-5, we investigate the effects of PFRDB while fixing the number of ResBlock at 20. We observe that adding more PFRDBs \cite{yi2019progressive} achieve a small but consistent performance improvement. However, introduction of PFRDBs requires more computational cost and much training time. So we use 5 PFRDBs to learn more spatial-temporal information by leveraging low- and high-level features.

Besides, we compare cases 6-10 to study the effects of ResBlock when the number of ResBlock is fixed at 5. It can show that we achieve a marginal performance gain when adding more ResBlocks. This suggests that we can achieve robust representation ability while maintaining relatively small network size. To balance the trade-off between computational cost and time, we adopt 20 ResBlocks here. 

Overall, our MEGAN can make superior improvements including 5 PFRDBs and 20 ResBlocks. Using the proposed LMGA module, our MEGAN can better handle complex dynamic space-time scenes

% When comparing cases 2, 4, and 7, we learn that more non-local blocks achieve better results. However, the introduction of non-local block consumes much time. So we use 2 non-local blocks by considering low- and high-level features. When RNAB number is fixed in cases 5 and 7 or cases 6 and 8, performance also benefits from more RABs.
